# Supplementary material for: Grant-Free Random Access of IoT devices in Massive MIMO with Partial CSI
Source: arXiv:2301.04861 source file (2023-01-12)
Supplement: Supplementary file 1 [file Appendix.tex]

\section{Appendix}
\label{section:appendix}
\TODO{}

Using the differential rule $\partial (\log |\mat{A}|)=\tr[\mat{A}^{-1} \partial \mat{A}]$, the derivative of $\tilde{f}(r_{k'})$  in (\ref{eq:f_r_k_prime}) is 
\begin{align*}
	\frac{d\tilde{f}}{dr_{k'}}&=-M \tr[\mat{C}^{-1} 2\vect{s}_k \vect{s}_k^H \lambda_k^2r_{k'}]+\frac{(2\alpha r_{k'}+\beta)(1+\delta r_{k'}^2)-(\alpha r_{k'}^2+\beta r_{k'})2\delta r_{k'}}{\left(1+\delta r_{k'}^2\right)^2}\\
% 	&=-2M\lambda_k^2 \vect{s}_k^H\mat{C}^{-1} \vect{s}_k r_{k'}+\frac{(2\alpha r_{k'}+\beta)(1+\delta r_{k'}^2)-(\alpha r_{k'}^2+\beta r_{k'})2\delta r_{k'}}{\left(1+\delta r_{k'}^2\right)^2}\\
	&=-2M\lambda_k^2 \vect{s}_k^H\mat{C}^{-1} \vect{s}_k r_{k'}+\frac{-r_{k'}^2\beta\delta+r_{k'}2\alpha+\beta}{\left(1+\delta r_{k'}^2\right)^2}.
\end{align*}
Applying, again, the Sherman-Morisson formula (\ref{eq:C_inverse_s_Sherman_Morrison_formula}) gives
\begin{align}\label{eq:derivitive_ampl}
	\frac{d\tilde{f}}{dr_{k'}}%&=-2M\lambda_k^2 \frac{\vect{s}_k^H\mat{C}_{-k'}^{-1}\vect{s}_{k'}}{1+\vect{s}_{k'}^H\mat{C}_{-k'}^{-1}\vect{s}_{k'}r_{k'}^2\lambda_{k'}^2} r_{k'}+\frac{-r_{k'}^2\beta\delta+r_{k'}2\alpha+\beta}{\left(1+\delta r_{k'}^2\right)^2}\\
	&=-2M \frac{\delta r_{k'}}{1+\delta r_{k'}^2} +\frac{-r_{k'}^2\beta\delta+r_{k'}2\alpha+\beta}{\left(1+\delta r_{k'}^2\right)^2}.
\end{align}
